# Supplementary material for: Symmetries of weighted networks: weight approximation method and its application to food webs
Source: arXiv:2506.11824 ancillary file (2026-06-18)
Supplement: Supplementary file 1 [file Symmetries_JulKol_MatIsk_Sup_Mat_Food_Web_Dataset.pdf]

## Appendix A

# Food web dataset - Supplementary Material to "Symmetries of weighted networks: weight approximation method and its application to food webs"

References to the sources of empirical food webs used.

| Name                           | Ecobase<br>ID /<br>Re-<br>marks | Reference                                                                                                                                                                                                                                       |
|--------------------------------|---------------------------------|-------------------------------------------------------------------------------------------------------------------------------------------------------------------------------------------------------------------------------------------------|
| Aggregated Flow<br>Model       |                                 | Baird, D., McGlade, J. M., Ulanowicz, R. E. The comparative ecology of six marine ecosystems. Philos. Trans. - R. Soc. London, B 333, 15–29 (1991). <a href="https://doi.org/10.1098/rstb.1991.0058">https://doi.org/10.1098/rstb.1991.0058</a> |
| Benguela up-<br>welling system |                                 |                                                                                                                                                                                                                                                 |
| Ems Estuary                    |                                 |                                                                                                                                                                                                                                                 |

**References to the sources of empirical food webs used - continued from previous page**

| <b>Name</b>                  | <b>Ecobase ID / Re-marks</b> | <b>Reference</b>                                                                                                                                                                                                                                                                                     |
|------------------------------|------------------------------|------------------------------------------------------------------------------------------------------------------------------------------------------------------------------------------------------------------------------------------------------------------------------------------------------|
| Peruvian Up-welling          |                              |                                                                                                                                                                                                                                                                                                      |
| Alaska, Prince William Sound | 2                            | Dalsgaard, J., Pauly, D., Okey, T. A. Preliminary mass-balance model of Prince William Sound, Alaska, for the pre-spill period, 1980-1989 Fisheries Centre Research Reports 5 (2) (1997) doi: <a href="http://dx.doi.org/10.14288/1.0074775">http://dx.doi.org/10.14288/1.0074775</a>                |
| Albatross Bay                | 465                          | Okey, T.A. A trophodynamic ecosystem model of Albatross Bay, Gulf of Carpentaria: revealing a plausible fishing explanation for prawn catch declines. CSIRO Marine and Atmospheric Research Paper (2006).                                                                                            |
| Aleutian Islands             | 252                          | Gu  nette, S., Heymans, S.J.J., Christensen, V., Trites, A. W. Ecosystem models show combined effects of fishing, predation, competition, and ocean productivity on Steller sea lions ( <i>Eumetopias jubatus</i> ). Alaska Canadian Journal of Fisheries and Aquatic Sciences 63, 2495-2517 (2006). |
| South East Alaska            | 438                          |                                                                                                                                                                                                                                                                                                      |
| Alto Golfo de California     | 242                          | Morales-Z  rate, M. V., Arregu  n-S  nchez, F., L  pez-Martinez, J., Lluch-Cota, S. E. Ecosystem trophic structure and energy flux in the Northern Gulf of California M  xico. Ecological Modelling 174, 331-345 (2004) 10.1016/j.ecolmodel.2003.09.028                                              |
| Antarctic                    | 447                          | Hoover, C. Ecosystem effects of climate change in the Antarctic Peninsula. Ecopath 25 years conference proceedings: Extended abstracts, 96-97 (2009).                                                                                                                                                |
| Arachania                    | 567                          | Lercari, D., Bergamino, L., Defeo, O. Trophic models in sandy beaches with contrasting morphodynamics: comparing ecosystem structure and biomass flow. Ecological Modelling. 221, 2751-2759 (2010) 10.1016/j.ecolmodel.2010.08.027.                                                                  |
| Barra Del Chuy               | 568                          |                                                                                                                                                                                                                                                                                                      |
| Australia North West Shelf   | 405                          | Bulman, C. Trophic webs and modelling of Australias North West Shelf. CSIRO Mar. Atmosp. Res.. 53-57 (2006).                                                                                                                                                                                         |
| Azores archipelago           | 7                            | Gu  nette, S., Morato, T. The Azores Archipelago, 1997 Fisheries Impacts on North Atlantic Ecosystems: Models and Analyses. Fisheries Centre research reports, 9, 4, 241-270 (2001).                                                                                                                 |
| Baja California              | 417                          | Cisneros-Montemayor, A. M., Christensen, V., Arregu  n-S  nchez, F., Sumaila, R. U. Ecosystem models for management advice: An analysis of recreational and commercial fisheries policies in Baja California Sur Mexico. Ecological Modelling 228, 8-16 (2012).                                      |
| Baltic Ecosystem             |                              | Wulff, F., Ulanowicz, R. A comparative anatomy of the Baltic Sea and Chesapeake Bay. Network Analysis in Marine Ecology 32, 232-256                                                                                                                                                                  |
| Bamboung                     | 179                          | Coll  ter, M., Gascuel, D., Ecoutin, J.-M., Tito de Morais, L. Modelling trophic flows in ecosystems to assess the efficiency of marine protected area (MPA), a case study on the coast of Senegal. Ecological Modelling 232, 1-13, DOI:10.1016/j.ecolmodel.2012.01.019                              |
|                              | 180                          |                                                                                                                                                                                                                                                                                                      |

**References to the sources of empirical food webs used - continued from previous page**

| Name                   | Ecobase ID / Re-marks | Reference                                                                                                                                                                                                                                                                                                                                      |
|------------------------|-----------------------|------------------------------------------------------------------------------------------------------------------------------------------------------------------------------------------------------------------------------------------------------------------------------------------------------------------------------------------------|
| Barents Sea            | 63                    | Blanchard, J. L., Pinnegar, J. K., Mackinson, S. Exploring Marine Mammal-Fishery Interactions Using Ecopath with Ecosim: Modelling the Barents Sea Ecosystem. Science Series Technical Report 117 (2002).                                                                                                                                      |
| Low Barents Sea        | 64                    |                                                                                                                                                                                                                                                                                                                                                |
| Bay of Biscay          | 335                   | Lassalle, G., Gascuel, D., Lobry, J., Pierce, G. J. Ridoux, V., Santos, M.B., Spitz, J., Niquil, N. An ecosystem approach for the assessment of fisheries impacts on marine top predators: the Bay of Biscay case study. ICES Journal of Marine Science: Journal du Conseil. 69, 6, 925-938                                                    |
| Bay of Biscay          | 633                   | Ainsworth, C., Feriss, B., Leblond, E., Gu  nette, S. The Bay of Biscay, France: 1998 and 1970 models. Fisheries Impacts on North Atlantic Ecosystems: Models and Analyses. 271-313                                                                                                                                                            |
|                        | 634                   |                                                                                                                                                                                                                                                                                                                                                |
| Black Sea              | 435                   | Gucu, A. C. Can Overfishing be Responsible for the Successful Establishment of Mnemiopsis leidyi in the Black Sea? Estuarine, Coastal and Shelf Science. 439-451                                                                                                                                                                               |
|                        | 433                   |                                                                                                                                                                                                                                                                                                                                                |
| Black Sea              | 691                   | Akoglu, E., Salihoglu, B., Libralato, S., Oguz, T., Solidoro, C. An indicator-based evaluation of Black Sea food web dynamics during 1960-2000. Journal of Marine Systems 134, 113-125, (2004). <a href="https://doi.org/10.1016/j.jmarsys.2014.02.010">https://doi.org/10.1016/j.jmarsys.2014.02.010</a>                                      |
|                        | 692                   |                                                                                                                                                                                                                                                                                                                                                |
|                        | 693                   |                                                                                                                                                                                                                                                                                                                                                |
| Black Sea              | 468                   | Orek, H., Gucu, A. C., Bingel, F. An application of mass balance Ecopath model to the trophic structure in the Black Sea after anchovy collapse. Oceanography of the Eastern Mediterranean and Black Sea (Ay  en Yilmaz ed.), 119 (T  B  TAK Publishers, 2003).                                                                                |
| Bolinao Coral Reef     | 682                   | Ali  o, P. M., McManus, L. T., McManus, J. W., Na  ola Jr, C. L., Fortes, M. D., Trono Jr. G.C., Jacinto, G.S. Initial parameter estimations of a coral reef flat ecosystem in Bolinao, Pangasinan, Northwestern Philippines. in Trophic models of aquatic ecosystems. ICLARM Conf. Proc. (D. Pauly and V. Christensen ed.) 26, 252-258 (1993) |
| Bothnian Bay           |                       | Sandberg, J., Elmgren R., Wulff, F. Carbon flows in Baltic Sea food webs—a re-evaluation using a mass balance approach. Journal of Marine Systems 25 (3-4), 249-260 (2000).                                                                                                                                                                    |
| Bothnian Sea           |                       |                                                                                                                                                                                                                                                                                                                                                |
| British Columbia Coast | 478                   | Preikshot, D. B. The influence of geographic scale, climate and trophic dynamics upon North Pacific oceanic ecosystem models (Doctoral dissertation, University of British Columbia). DOI: 10.14288/1.0074902 (2007)                                                                                                                           |
| North East Pacific     | 479                   |                                                                                                                                                                                                                                                                                                                                                |
| Strait of Georgia      | 477                   |                                                                                                                                                                                                                                                                                                                                                |
| Calvi Bay              | 473                   | Pinnegar, J. K., Polunin, N. V. C. Predicting indirect effects of fishing in Mediterranean rocky littoral communities using a dynamic simulation model. Ecological Modelling 172 (2-4), 249-267 (2004).                                                                                                                                        |

**References to the sources of empirical food webs used - continued from previous page**

| <b>Name</b>                         | <b>Ecobase ID / Re-marks</b> | <b>Reference</b>                                                                                                                                                                                                                                      |
|-------------------------------------|------------------------------|-------------------------------------------------------------------------------------------------------------------------------------------------------------------------------------------------------------------------------------------------------|
| Campeche                            | 323                          | Vega-Cendejas, M. E., Arreguin-Sánchez, F., Hernández, M. Trophic fluxes on the Campeche Bank, Mexico. Trophic models of aquatic ecosystems. ICLARM Conf. Proc. 26, 206-213 (1993).                                                                   |
| Canada, Grand Banks of Newfoundland | 655                          | Bundy, A. Adaptation of a Newfoundland-Labrador Ecopath model for 1985-1987 in statistical area 2J3KLNO to the area 2J3KL. Fisheries Centre Research Reports 10, 1, 13-21 (2002).                                                                     |
| Cape Verde                          | 486                          | Stobberup, K. A., Ramos, V.D.M., Coelho, M. L. Ecopath model of the Cape Verde coastal ecosystem. West African marine ecosystems: models and fisheries impacts. Fisheries Center Research Reports. 12, 39-56 (2004).                                  |
| Sylt-Romo Bight                     | Carbon Network               | Baird, D. et al. Energy flow of a boreal intertidal ecosystem, the Sylt-Rømø Bight. Marine Ecology-progress Series 279, 45-61 (2004).                                                                                                                 |
| Chesapeake Bay                      | Carbon Mesohaline            | Baird, D., Ulanowicz, R. The seasonal dynamics of the Chesapeake Bay ecosystem. Ecol. Monogr. 59, 329-364 (1989)                                                                                                                                      |
| Caribbean                           | 24                           | Melgo, J. L., Morissette, L., Kaschner, K., Gerber, L. Modelling the trophic role of marine mammals in tropical areas: data requirements, uncertainty, and validation. Fisheries Center Research Reports 17 (2) 53-120 (2009)                         |
| Celestun                            | 246                          | Chávez, E. A., Garduño, M., Arreguin-Sánchez, F. Trophic Dynamic Structure of Celestun lagoon, Southern Gulf of Mexico. in Trophic models of aquatic ecosystems. ICLARM Conf. Proc. (D. Pauly and V. Christensen ed.) 26, 186-192 (1993)              |
| Celestun mangrove                   | 247                          | Vega-Cendejas, M. E., Arreguin-Sánchez, F. Energy fluxes in a mangrove ecosystem from a coastal lagoon in Yucatan Peninsula, Mexico. Ecological Modelling 137, 119-133 (2001) 10.1016/S0304-3800(00)00421-X.                                          |
| Central Atlantic                    | 28                           | Vasconcellos, M., Watson, R. Mass-balance models of oceanic systems in the Atlantic. in West African marine ecosystems: models and fisheries impacts (M.L.D. Palomares and D. Pauly ed.) 171-214 (2004).                                              |
|                                     | 29                           |                                                                                                                                                                                                                                                       |
| North Atlantic                      | 111                          |                                                                                                                                                                                                                                                       |
|                                     | 112                          |                                                                                                                                                                                                                                                       |
| Central Baltic Sea                  | 608                          | Tomczak, M. T., Niiranen, S., Hjerne, O., Blenckner, T. Ecosystem flow dynamics in the Baltic Proper—Using a multi-trophic dataset as a basis for food-web modelling. Ecological Modelling 230, 123-147 (2012). doi: 10.1016/j.ecolmodel.2011.12.014. |
| Central Chile                       | 637                          | Neira, S., Arancibia, H., Cubillos, L. Comparative analysis of trophic structure of commercial fishery species off Central Chile in 1992 and 1998. Ecological Modelling 172, 233-248 (2004). doi: 10.1016/j.ecolmodel.2003.09.009.                    |

**References to the sources of empirical food webs used - continued from previous page**

| Name                       | Ecobase ID / Re-marks | Reference                                                                                                                                                                                                                                                                                                                                                                                              |
|----------------------------|-----------------------|--------------------------------------------------------------------------------------------------------------------------------------------------------------------------------------------------------------------------------------------------------------------------------------------------------------------------------------------------------------------------------------------------------|
| Central Gulf of California | 239                   | Arreguin-Sánchez, F., Arcos, E., Chávez, E. A. Flows of biomass and structure in an exploited benthic ecosystem in the Gulf of California, Mexico. Ecological Modelling 156, 167-183 (2002). doi: 10.1016/S0304-3800(02)00159-X.                                                                                                                                                                       |
| Chesapeake                 | 34                    | Christensen, V., Beattie, A., Buchanan, C., Hongguang, M., Martell, S.J.D., Latour, R.J., Preikshot, D., Sigrist, M.B., Uphoff, J.H., Walters, C.J., Wood, R.J., Townsend, H. Fisheries Ecosystem Model of the Chesapeake Bay: Methodology, Parameterization, and Model Exploration. NOAA Technical Memorandum NMFS-F-SPO (2009).                                                                      |
| Crystal River Creek        | Control               | Homer, M., Kemp, W. M. Unpublished Ms. See also Ulanowicz, R.E. Growth and Development: Ecosystems Phenomenology. (Springer, New York) 69-79. (1986).                                                                                                                                                                                                                                                  |
|                            | Delta Temp            |                                                                                                                                                                                                                                                                                                                                                                                                        |
| Cypress                    | Dry Season            | Ulanowicz, R. E., Bondavalli, C. and, Egnotovitch M. S. Network analysis of trophic dynamics in South Florida ecosystems, FY 96: the cypress wetland ecosystem. Annual Report to the United States Geological Service Biological Resources Division, University of Miami Coral Gables, [UMCES] CBL 97-075, Maryland System Center for Environmental Science, Chesapeake Biological Laboratory. (1997). |
|                            | Wet Season            |                                                                                                                                                                                                                                                                                                                                                                                                        |
| Danajon Bank               | 711                   | Bacalso, R.T.M., Wolff, M. Trophic flow structure of the Danajon ecosystem (Central Philippines) and impacts of illegal and destructive fishing practices Journal of Marine Systems 139, 103-118 (2014).                                                                                                                                                                                               |
| Denmark, Faroe Islands     | 46                    | Zeller, D., Reinert, J. Modelling spatial closures and fishing effort restrictions in the Faroe Islands marine ecosystem Ecological Modelling 172, 403-420 (2004). 10.1016/j.ecolmodel.2003.09.020                                                                                                                                                                                                     |
| Durban Eddy                | Summer C              | Scharler, U. M., Ayers, M., de Lecea, A., Pretorius, M., Fennessy S., Huggett J., MacKay C., Muir, D. Riverine influence determines nearshore heterogeneity of nutrient (C, N, P) content and stoichiometry in the KwaZulu-Natal Bight, South Africa. African J. Mar. Sci. 38, S193–S203 (2016). 10.2989/1814232X.2016.1150347.                                                                        |
|                            | Summer N              |                                                                                                                                                                                                                                                                                                                                                                                                        |
|                            | Summer P              |                                                                                                                                                                                                                                                                                                                                                                                                        |
|                            | Winter C              |                                                                                                                                                                                                                                                                                                                                                                                                        |
|                            | Winter N              |                                                                                                                                                                                                                                                                                                                                                                                                        |
| Richards Bay               | Summer C              |                                                                                                                                                                                                                                                                                                                                                                                                        |

References to the sources of empirical food webs used - continued from previous page

| Name             | Ecobase ID / Re-marks | Reference                                                                                                                                                                                                                                                      |
|------------------|-----------------------|----------------------------------------------------------------------------------------------------------------------------------------------------------------------------------------------------------------------------------------------------------------|
|                  | Summer N              |                                                                                                                                                                                                                                                                |
|                  | Summer P              |                                                                                                                                                                                                                                                                |
|                  | Winter C              |                                                                                                                                                                                                                                                                |
|                  | Winter N              |                                                                                                                                                                                                                                                                |
|                  | Winter P              |                                                                                                                                                                                                                                                                |
| Thukela Mouth    | Summer C              |                                                                                                                                                                                                                                                                |
|                  | Summer N              |                                                                                                                                                                                                                                                                |
|                  | Summer P              |                                                                                                                                                                                                                                                                |
|                  | Winter C              |                                                                                                                                                                                                                                                                |
|                  | Winter N              |                                                                                                                                                                                                                                                                |
|                  | Winter P              |                                                                                                                                                                                                                                                                |
| East Bass Strait | 406                   | Bulman, C., Condie, S., Furlani, D., Cahill, M., Klaer, N., Goldsworthy, S., Knuckey, I. Trophic dynamics of the eastern shelf and slope of the south east fishery: impacts of and on the fishery. Final Report for Fisheries Research and Development (2006). |
| East Kleinemonde | EK0306C               | Ortega-Cisneros, K., Scharler, U. M., Whitfield, A. K. Carbon and nitrogen system dynamics in three small South African estuaries, with particular emphasis on the influence of seasons, river flow and mouth state. Mar. Ecol. Prog. Ser. 557, 17–30 (2016).  |
|                  | EK0706C               |                                                                                                                                                                                                                                                                |
|                  | EK0906C               |                                                                                                                                                                                                                                                                |

**References to the sources of empirical food webs used - continued from previous page**

| Name                  | Ecobase ID / Re-marks | Reference                                                                                                                                                                                                                                                                                                                                                                                                                                                                                               |
|-----------------------|-----------------------|---------------------------------------------------------------------------------------------------------------------------------------------------------------------------------------------------------------------------------------------------------------------------------------------------------------------------------------------------------------------------------------------------------------------------------------------------------------------------------------------------------|
|                       | EK1106C               |                                                                                                                                                                                                                                                                                                                                                                                                                                                                                                         |
| Eastern Bering Sea    | 183                   | Trites, A. W., Livingston, P. A., Mackinson, S., Vasconcellos, M. C., Springer, A. M., Pauly, D. Ecosystem Change and the Decline of Marine Mammals the Eastern Bering Sea: Testing the Ecosystem Shift and Commercial Whaling Hypotheses. Fisheries Centre Research Reports 7, Fisheries Centre, University of British Columbia (1999). 10.14288/1.0348097                                                                                                                                             |
| Eastern Scotian Shelf | 40                    | Bundy, A. Mass balance models of the eastern Scotian Shelf before and after the cod collapse and other ecosystem changes. Canadian Technical Report of Fisheries and Aquatic Sciences (Dartmouth - Nova Scotia, Fisheries and Oceans Canada) 1488-5379 (2004).                                                                                                                                                                                                                                          |
|                       | 41                    |                                                                                                                                                                                                                                                                                                                                                                                                                                                                                                         |
| EMAX-GB               |                       | Link, J., Overholtz, W., O'Reilly, J., Green, J., Dow, D., Palka, D., Legault, C., Vitaliano, J., Guida, V., Fogarty, M., Brodziak, J., Methratta, L., Stockhausen, W., Col, L., Griswold, C. The northeast US continental shelf energy modeling and analysis exercise (EMAX): Ecological network model development and basic ecosystem metrics. J. Mar. Syst. 74, 453-474 (2008) <a href="http://www.nefsc.noaa.gov/publications/crd/crd0615/">http://www.nefsc.noaa.gov/publications/crd/crd0615/</a> |
| EMAX-GOM              |                       |                                                                                                                                                                                                                                                                                                                                                                                                                                                                                                         |
| EMAX-MAB              |                       |                                                                                                                                                                                                                                                                                                                                                                                                                                                                                                         |
| EMAX-SNE              |                       |                                                                                                                                                                                                                                                                                                                                                                                                                                                                                                         |
| Eritrea               | 496                   | Tsehaye, I., Nagelkerke, L. A. J. Exploring optimal fishing scenarios for the multispecies artisanal fisheries of Eritrea using a trophic model. Ecological Modelling 212, 319-333 (2008).                                                                                                                                                                                                                                                                                                              |
| Everglades Graminoids | Dry Season            | Ulanowicz, R. E., Heymans, J. J., Egnotovitch, M. S. Network Analysis of Trophic Dynamics in South Florida Ecosystems, FY 99: The Graminoid Ecosystem. Annual Report to the United States Geological Service Biological Resources Division Ref. No.[UMCES] CBL 00-0176, Chesapeake Biological Laboratory, University of Maryland (2000).                                                                                                                                                                |
|                       | Wet Season            |                                                                                                                                                                                                                                                                                                                                                                                                                                                                                                         |
| Falkland Islands      | 411                   | Cheung, W.W.L., Pitcher, T. J. A mass-balance model of the Falkland Islands fisheries and ecosystems. Modeling Antarctic Marine Ecosystems, 65-84 (2005).                                                                                                                                                                                                                                                                                                                                               |
| Narragansett Bay      | 08/01/94              | Monaco, M. E., Ulanowicz, R. E. 1997. Comparative ecosystem trophic structure of three U.S. Mid-Atlantic estuaries. Mar. Ecol. Prog. Ser. 161, 239-254.                                                                                                                                                                                                                                                                                                                                                 |
| Narragansett Bay      | 08/01/94              |                                                                                                                                                                                                                                                                                                                                                                                                                                                                                                         |
| Florida Bay           | Dry Season            | Ulanowicz, R. E., Bondavalli, C., Egnotovitch, M. S. 1998. Network Analysis of Trophic Dynamics in South Florida Ecosystem, FY 97: The Florida Bay Ecosystem. Annual Report to the United States Geological Service Biological Resources Division Ref. No. [UMCES]CBL 98-123. Chesapeake Biological Laboratory, Solomons, MD 20688-0038 USA. <a href="http://cbl.umces.edu/~atlss/FBay701.html">http://cbl.umces.edu/~atlss/FBay701.html</a>                                                            |
|                       | Wet Season            |                                                                                                                                                                                                                                                                                                                                                                                                                                                                                                         |

**References to the sources of empirical food webs used - continued from previous page**

| Name                           | Ecobase ID / Re-marks | Reference                                                                                                                                                                                                                                                                                                                                                                                   |
|--------------------------------|-----------------------|---------------------------------------------------------------------------------------------------------------------------------------------------------------------------------------------------------------------------------------------------------------------------------------------------------------------------------------------------------------------------------------------|
| Galapagos, Floreana Rocky Reef | 48                    | Okey, T. A., Banks, S., Born, A. F., Bustamante, R. H., Calvopiña, M., Edgar, G.J., Espinoza, E., Fariña, J.M., Garske, L.E., Reck, G.K., Salazar, S., Shepherd, S., Toral-Granda, V., Wallem, P. A trophic model of a Galápagos subtidal rocky reef for evaluating fisheries and conservation strategies. <i>Ecological Modelling</i> 172, 383-401 (2004). 10.1016/j.ecolmodel.2003.09.019 |
| Garonne                        | 221                   | Palomares, M.L.D., Yulianto, B., Puy, L., Bengen, D., Belaud, A. A Preliminary Model of the Garonne River (Toulouse, France) Ecosystem in Spring. In <i>Trophic Models of Aquatic Ecosystems</i> 26, 172-179 (1993).                                                                                                                                                                        |
| Georges Bank                   | 705                   | Link, J. S., Griswold, C. A., Methratta, E. T., Gunnard, J. Documentation for the Energy Modeling and Analysis eXercise (EMAX). Northeast Fish. Sci. Cent. Ref. Doc. (2006).                                                                                                                                                                                                                |
| Gulf of Maine                  | 704                   |                                                                                                                                                                                                                                                                                                                                                                                             |
| Mid-Atlantic Bight             | 707                   |                                                                                                                                                                                                                                                                                                                                                                                             |
| Southern New England           | 706                   |                                                                                                                                                                                                                                                                                                                                                                                             |
| Germany, Schlei Fjord          | 464                   | Christensen, V., Pauly, D. The ECOPATH II - a software for balancing steady-state ecosystem models and calculating network characteristics. <i>Ecological Modelling</i> 61. 169-185. (1992). 10.1016/0304-3800(92)90016-8.                                                                                                                                                                  |
| Gironde estuary                | 218                   | Lobry, J. Which reference pattern of functioning for estuarine ecosystems? The case of fish successions in the Gironde estuary (2004).                                                                                                                                                                                                                                                      |
| Golfo Dulce                    | 53                    | Wolff, M., Hartmann, H. J., Koch, V. A pilot trophic model for Golfo Dulce, a fjord-like tropical embayment, Costa Rica. <i>Revista de Biología Tropical</i> 44, 215-231 (1996).                                                                                                                                                                                                            |
| Grand Banks of Newfoundland    | 105                   | Heymans, J. J., Pitcher, T. A Picasso-esque View of the Marine Ecosystem of Newfoundland and Southern Labrador: Models for the Time Periods 1450 and 1900 Ecosystem models of Newfoundland for the time periods 1995, 1985, 1900 and 1450. <i>Fisheries Centre Research Reports</i> , 10 (5), 44-73 (2002).                                                                                 |
| Grand Banks of Newfoundland    | 107                   | Heymans, J. J. Ecosystem models of Newfoundland and Southeastern Labrador: Additional information and analyses for Back to the Future. <i>Fisheries Centre Research Reports</i> 11 (5), 79 pp. (2003). 10.14288/1.0074790                                                                                                                                                                   |
|                                | 108                   |                                                                                                                                                                                                                                                                                                                                                                                             |
| Greenland, West Coast          | 168                   | Pedersen, S. A. Zeller, D. A mass balance model for the West Greenland marine ecosystem. In: <i>Fisheries Impacts on North Atlantic Ecosystems: Models and Analyses.</i> ( Guénette S., Christensen, V., Pauly, D. ed.) 111-127 (University of British Columbia, Vancouver, 2001).                                                                                                          |
| Guinea                         | 646                   | Guénette, S., Diallo, I. Addendum: Modèles de la côte guinéenne, 1985 et 1998. <i>West African marine ecosystems: models and fisheries impacts.</i> <i>Fisheries Centre Research Reports</i> , 12 (7), 124-159 (2004). 10.14288/1.0074805                                                                                                                                                   |

**References to the sources of empirical food webs used - continued from previous page**

| <b>Name</b>               | <b>Ecobase ID / Re-<br/>marks</b> | <b>Reference</b>                                                                                                                                                                                                                                                                                                                                                                                                      |
|---------------------------|-----------------------------------|-----------------------------------------------------------------------------------------------------------------------------------------------------------------------------------------------------------------------------------------------------------------------------------------------------------------------------------------------------------------------------------------------------------------------|
| Guinea                    | 725                               | Gascuel, D., Guénette, S., Diallo, I., Sidibé, A. Impact de la pêche sur l'écosystème marin de Guinée - Modélisation EwE 1985/2005. Fisheries Centre Research Reports 17 (4), (2009).                                                                                                                                                                                                                                 |
|                           | 726                               |                                                                                                                                                                                                                                                                                                                                                                                                                       |
| Gulf of California        | 450                               | Lercari, D., Arreguín-Sánchez, F. An ecosystem modelling approach to deriving viable harvest strategies for multispecies management of the Northern Gulf of California. Aquatic Conserv: Mar. Freshw. Ecosyst., 19: 384-397. (2009). doi:10.1002/aqc.978                                                                                                                                                              |
| Gulf of Carpentaria       | 466                               | Okey, T. A. Griffiths, S., Pascoe, S., Kenyon, R., Miller, M., Dell, Q., Pillans, R., Buckworth, R.C., Gribble, N., Engstrom, N., Bishop, J., Milton, D., Salini, J., Stevens, J. The effect of illegal foreign fishing on the ecosystem in the Gulf of Carpentaria: management options and downstream effects on other fisheries. Final Report to Australian Fisheries Management Authority Project 2006/825 (2007). |
| Gulf of Maine             | 444                               | Heymans, J. J. The Gulf of Maine, 1977-1986 Fisheries Impacts on North Atlantic Ecosystems: Models and Analyses. 129-149 (2001).                                                                                                                                                                                                                                                                                      |
| Gulf of Mexico            | 520                               | Walters, C., Martell, S.J.D., Christensen, V., Mahmoudi, B. An Ecosim Model for Exploring Gulf of Mexico Ecosystem Management Options: Implications of Including Multistanza Life-History Models for Policy Predictions. Bulletin of Marine Science 83, 251-271 (2008).                                                                                                                                               |
| Tampa Bay                 | 153                               |                                                                                                                                                                                                                                                                                                                                                                                                                       |
| Gulf of Mexico            | 58                                | Browder, J. A. Browder, J. A. A pilot model of the Gulf of Mexico continental shelf . In Trophic models of aquatic ecosystems. ICLARM Conference Proceedings, 26 (390), 279-284 (1993).                                                                                                                                                                                                                               |
| Gulf of Nicoya            | 677                               | Wolff, M., Chavarria, J. B. Koch, V., Vargas, J. A. A trophic flow model of the Golfo de Nicoya, Costa Rica. Revista de Biología Tropical, 63-79 (1998).                                                                                                                                                                                                                                                              |
| Gulf of Salamanca         | 669                               | Duarte, L. O., Garcia, C. B. Trophic role of small pelagic fishes in a tropical upwelling ecosystem Ecological Modelling 172 (2-4), 323-338 (2004).                                                                                                                                                                                                                                                                   |
| Gulf of Thailand          | 412                               | Christensen, V. Fishery-induced changes in a marine ecosystem: insight from models of the Gulf of Thailand. Journal of Fish Biology 53, 128-142 (1998).                                                                                                                                                                                                                                                               |
| Hudson Bay                | 446                               | Hoover, C. Hudson Bay ecosystem: past, present, and future. In A Little Less Arctic , 217-236 (Springer, Dordrecht, 2010).                                                                                                                                                                                                                                                                                            |
| Huizache-Caimanero        | 241                               | Zetina-Rejón, M. J. Arreguín-Sánchez, F., Chávez, E. A. Trophic structure and flows of energy in the Huizache-Caimanero lagoon complex on the Pacific coast of Mexico. Estuarine, Coastal and Shelf Science 57, 803-815 (2003).                                                                                                                                                                                       |
| Humboldt Current          | 487                               | Tam, J., Taylor, M. H., Blaskovic, V., Espinoza, P., Michael Ballón, R., Díaz E., Wosnitza-Mendo, C., Argüelles, J., Purca, S., Ayón P. Trophic modeling of the Northern Humboldt current ecosystem, Part I: comparing trophic linkages under La Niña and El Niño conditions. Progress in Oceanography 79, 352-365 (2008).                                                                                            |
| Northern Humboldt Current | 488                               |                                                                                                                                                                                                                                                                                                                                                                                                                       |

**References to the sources of empirical food webs used - continued from previous page**

| <b>Name</b>              | <b>Ecobase ID / Re-marks</b> | <b>Reference</b>                                                                                                                                                                                                                                                                                                                         |
|--------------------------|------------------------------|------------------------------------------------------------------------------------------------------------------------------------------------------------------------------------------------------------------------------------------------------------------------------------------------------------------------------------------|
| Iceland                  | 227                          | Buchary, E. A. Preliminary reconstruction of the Icelandic marine ecosystem in 1950 and some predictions with time series data Fisheries Centre Research Reports, 9 (5) 198-206 (2001).                                                                                                                                                  |
| Icelandic shelf          | 68                           | Samb B.(1999). Icelandic Shelf                                                                                                                                                                                                                                                                                                           |
| Independence Bay         | 490                          | Taylor, M. H., Wolff, M., Mendo, J., Yamashiro, C. Changes in trophic flow structure of Independence Bay over an ENSO cycle. Progress in Oceanography 79, 336-351 (2008). (Peru).                                                                                                                                                        |
| Irish Sea                | 448                          | Lees, K., Mackinson, S. An Ecopath model of the Irish Sea: ecosystems properties and sensitivity analysis. Cefas Science Series Technical Report 138 (2007).                                                                                                                                                                             |
| Jalisco and Colima Coast | 307                          | Galván Piña, V. H. Impacto de la pesca en la estructura, función y productividad del ecosistema de la Plataforma Continental de las costas de Jalisco y Colima, México. Doctoral dissertation, Instituto Politécnico Nacional. Centro Interdisciplinario de Ciencias Marinas (2005).                                                     |
| Jurien Bay               | 456                          | Lozano-Montes, H. M., Loneragan, N. R., Babcock, R. C., Jackson, K. Using trophic flows and ecosystem structure to model the effects of fishing in the Jurien Bay Marine Park, temperate Western Australia Marine and Freshwater Research, 62(5), 421-431 (2011).                                                                        |
| Kaloko Honokohau         | 499                          | Wabnitz, Colette C.C., Balazs G., Beavers, S., Bjorndal, K. A. , Bolten, A. B., Christensen, V., Hargrove, S., Pauly, D. Ecosystem structure and processes at Kaloko Honokōhau, focusing on the role of herbivores, including the green sea turtle Chelonia mydas, in reef resilience. Marine Ecology Progress Series 420, 27-44 (2010). |
| Kromme Estuary           | 04/01/00                     | Scharler, U. M., Baird, D. A comparison of selected ecosystem attributes of three South African estuaries with different freshwater inflow regimes, using network analysis. Journal of Marine Systems 56, 283-308 (2005).                                                                                                                |
| Sundays Estuary          | 04/01/00                     |                                                                                                                                                                                                                                                                                                                                          |
| Swartkops Estuary        | 04/01/00                     |                                                                                                                                                                                                                                                                                                                                          |
| Kuosheng Bay             | 266                          | Lin, H.-J., Shao, K.-T., Hwang, J.-S., Lo, W.-T., Cheng, I.-J., Lee, L.-H. A trophic model for Kuosheng Bay in northern Taiwan. Journal of Marine Science and Technology 12 (5), 424-432 (2004).                                                                                                                                         |
| Lagoon Chiku – Taiwan    | 267                          | Lin, H.-J., Shao, K.-T., Kuo, S.-R., Hsieh, H.-L., Wong, S.-L., Chen, I.-M., Lo, W.-T., Hung, J.-J. A Trophic Model of a Sandy Barrier Lagoon at Chiku in Southwestern Taiwan Estuarine, Coastal and Shelf Science 48 (5), 575-588 (1999).                                                                                               |
| Lake Michigan            | Control                      | Krause, A. Doctoral Dissertation, Michigan State University                                                                                                                                                                                                                                                                              |
| Lesser Antilles          | 459                          | Mohammed, E., Vasconcellos, M., Mackinson, S., Fanning, P., Heileman, S., Carocci F. Scientific Basis for Ecosystem-Based Management in the Lesser Antilles Including Interactions with Marine Mammals and Other Top Predators: A trophic model of the Lesser Antilles Pelagic Ecosystem. FI:GCP/RLA/140/JPN Technical Document (2008).  |

**References to the sources of empirical food webs used - continued from previous page**

| Name                               | Ecobase ID / Re-marks | Reference                                                                                                                                                                                                                                                                                                 |
|------------------------------------|-----------------------|-----------------------------------------------------------------------------------------------------------------------------------------------------------------------------------------------------------------------------------------------------------------------------------------------------------|
| Liberia                            | 513                   | Kay, D. W. Liberia report on Ecopath modeling. Ecosystem-based fisheries management using Ecopath with Ecosim (EwE) software. 105-118 (2011).                                                                                                                                                             |
| Looe Key National Marine Sanctuary | 269                   | McCormick Venier, J. Seasonal ecosystem models of the Looe Key National Marine Sanctuary, Florida. Doctoral dissertation, University of British Columbia (1997).                                                                                                                                          |
| Mangrove Estuary                   | Dry Season            | Ulanowicz, R. E., Bondavalli, C., Heymans, J. J., Egnotovich, M. S. 1999. Network analysis of trophic dynamics in South Florida ecosystems, FY 98: the mangrove ecosystem. Technical Report TS-191-99, Maryland System Center for Environmental Science, Chesapeake Biological Laboratory, Maryland, USA. |
|                                    | Wet Season            |                                                                                                                                                                                                                                                                                                           |
| Mauritania                         | 650                   | Ould Taleb Ould Sidi, M. M., Guénette, S. Modèle trophique de la ZEE mauritanienne: comparaison de deux périodes (1987 et 1998). West African marine ecosystems: models and fisheries impacts, 12-38 (2004).                                                                                              |
|                                    | 651                   |                                                                                                                                                                                                                                                                                                           |
| Mdloti Network                     | 12/01/02              | Scharler, U. M. Ecosystem development during open and closed phases of temporarily open/closed estuaries on the subtropical east coast of South Africa. Estuar. Coast. Shelf Sci. 108, 119–131 (2012).                                                                                                    |
|                                    | 06/01/02              |                                                                                                                                                                                                                                                                                                           |
|                                    | 03/01/02              |                                                                                                                                                                                                                                                                                                           |
|                                    | 03/01/02              |                                                                                                                                                                                                                                                                                                           |
|                                    | 09/01/02              |                                                                                                                                                                                                                                                                                                           |
| Mhlanga Network                    | 12/01/02              |                                                                                                                                                                                                                                                                                                           |
|                                    | 06/01/02              |                                                                                                                                                                                                                                                                                                           |
|                                    | 03/01/02              |                                                                                                                                                                                                                                                                                                           |
|                                    | 03/01/03              |                                                                                                                                                                                                                                                                                                           |
|                                    | 09/01/02              |                                                                                                                                                                                                                                                                                                           |
| Mauritanie                         | 689                   | Guenette, S., Meissa, B., Gascuel, D. Assessing the Contribution of Marine Protected Areas to the Trophic Functioning of Ecosystems: A Model for the Banc d'Arguin and the Mauritanian Shelf. PLoS One 9 (4), 1-16 (2014).                                                                                |
| Miramare                           | 452                   | Libralato, S., Tempesta, M., Solidoro, C., Spoto, M. An ecosystem model applied to Miramare Natural Marine Reserve: limits, advantages and perspectives. Biologia marina mediterranea 13 (1) 386-395 (2006).                                                                                              |
| Mondego Estuary                    | Zostrea site          | Patricio, J. Master's Thesis. University of Coimbra, Coimbra, Portugal.                                                                                                                                                                                                                                   |

**References to the sources of empirical food webs used - continued from previous page**

| <b>Name</b>    | <b>Ecobase ID / Re-marks</b> | <b>Reference</b>                                                                                                                                                                                                                                                                                                                 |
|----------------|------------------------------|----------------------------------------------------------------------------------------------------------------------------------------------------------------------------------------------------------------------------------------------------------------------------------------------------------------------------------|
| Morocco        | 654                          | Stanford, R., Lunn, K., Guénette, S. A preliminary ecosystem model for the Atlantic coast of Morocco for the mid-1980s. Fisheries Centre Research Reports, 9 (4), 314-344 (2001).                                                                                                                                                |
| NeuseEstuary   | Early Summer 1997            | Christian, R. R., Dame, J. K., Johnson, G., Peterson, C. H., Baird, D. Monitoring and modeling of the Neuse River Estuary, Phase 2: Functional assessment of environmental phenomena through network analysis. Report of Water Resources Research Institute of the University of North Carolina, UNC-WRRI 2004-343-E, 93 (2004). |
|                | Late Summer 1997             |                                                                                                                                                                                                                                                                                                                                  |
|                | Early Summer 1998            |                                                                                                                                                                                                                                                                                                                                  |
|                | Late Summer 1998             |                                                                                                                                                                                                                                                                                                                                  |
| New Foundland  | 518                          | Ainsworth, C. H., Sumaila, R. U. Intergenerational valuation of fisheries resources can justify long-term conservation: a case study in Atlantic cod ( <i>Gadus morhua</i> ). Canadian Journal of Fisheries and Aquatic Sciences 62 (5), 1104-1110 (2005).                                                                       |
| Ningaloo       | 432                          | Jones, T., Fulton, E. A., Wood, D. Challenging tourism theory through integrated models: how multiple model projects strengthen outcomes through a case study of tourism development on the Ningaloo Coast of Western Australia. MODSIM 2011 - 19th International Congress on Modelling and Simulation. 3112-3120 (2011).        |
| North Aegean   | 495                          | Tsagarakis, K., Coll, M., Giannoulaki, M., Somarakis, S., Papaconstantinou, C., Machias A. Food-web traits of the North Aegean Sea ecosystem (Eastern Mediterranean) and comparison with other Mediterranean ecosystems. Estuarine, Coastal and Shelf Science 88 (2), 233-248 (2010).                                            |
| North Benguela | 500                          | Watermeyer, K. E., Shannon, L. J., Roux, J. P., Griffiths, C. L. Changes in the trophic structure of the northern Benguela before and after the onset of industrial fishing. African Journal of Marine Science 30 (2), 383-403 (2008).                                                                                           |
|                | 501                          |                                                                                                                                                                                                                                                                                                                                  |
|                | 502                          |                                                                                                                                                                                                                                                                                                                                  |
|                | 503                          |                                                                                                                                                                                                                                                                                                                                  |
| North Brazil   | 189                          | Wolff, M., Koch, V., Isaac, V. A Trophic Flow Model of the Caeté Mangrove Estuary (North Brazil) with Considerations for the Sustainable Use of its Resources Estuarine, Coastal and Shelf Science 50 (6), 789-803 (2000).                                                                                                       |

**References to the sources of empirical food webs used - continued from previous page**

| <b>Name</b>                         | <b>Ecobase<br/>ID /<br/>Re-<br/>marks</b> | <b>Reference</b>                                                                                                                                                                                                                                                                  |
|-------------------------------------|-------------------------------------------|-----------------------------------------------------------------------------------------------------------------------------------------------------------------------------------------------------------------------------------------------------------------------------------|
| North Sea                           | 413                                       | Christensen, V., Reck, G., Maclean, J. L. Proceedings of the INCO-DC Conference Placing Fisheries in their Ecosystem Context. ACP-EU Fisheries Research Report. 79-79 (2002).                                                                                                     |
| North Sea                           | 457                                       | Mackinson, S., Daskalov G.(2008).An ecosystem model of the North Sea to support an ecosystem approach to fisheries management: description and parameterisation. Cefas Science Series Technical Report 142, 196                                                                   |
| North Sea                           | 680                                       | Christensen, V. A Model of Trophic Interactions in the North Sea in 1981, the Year of the Stomach Dana. ICES, 1-28 (1995).                                                                                                                                                        |
| North South of<br>China Sea         | 410                                       | Cheung, W. L. Vulnerability of marine fishes to fishing: from global overview to the Northern South China Sea. Doctoral dissertation, University of British Columbia (2007).                                                                                                      |
| Northern<br>Benguela                | 115                                       | Heymans, S.J.J., Sumaila, R. U. Updated Ecosystem Model for the Northern Benguela Ecosystem, Namibia INCOFISH Ecosystem Models: Transiting from Ecopath to Ecospace. Fisheries Centre Research Reports 15 (6), 25-70. (2007).                                                     |
| Northern<br>Benguela up-<br>welling |                                           | Heymans, J. J., Baird, D. A carbon flow model and network analysis of the northern Benguela upwelling system, Namibia. Ecological Modelling 126 (1), 9-32 (2000)                                                                                                                  |
| Northern British<br>Columbia        | 674                                       | Ainsworth, C., Heymans, J. J., Pitcher, T. J., Vasconcellos, M. Ecosystem Models of Northern British Columbia for the Time Periods 2000, 1950, 1900 and 1750. Fisheries Centre Research Reports 10 (4) (2002).                                                                    |
|                                     | 675                                       |                                                                                                                                                                                                                                                                                   |
| Northern Califor-<br>nian Current   | 519                                       | Walters, C., Christensen, V., Walters, W., Rose, K. Representation of multistanza life histories in Ecospace models for spatial organization of ecosystem trophic interaction patterns. Bulletin of Marine Science 86 (2), 439-459 (2010).                                        |
| Northern Califor-<br>nian Current   | 521                                       | Field, J. Application of ecosystem-based fishery management approaches in the northern California Current. Doctoral dissertation University of Washington (2004).                                                                                                                 |
| Northern Gulf of<br>St Lawrence     | 462                                       | Savenkoff, C., Bourdages, H., Castonguay, M., Morissette, L., Chabot, D., Hammill, M.O. Input data and parameter estimates for ecosystem models of the northern Gulf of St. Lawrence (mid-1990s). Canadian Technical Report of Fisheries and Aquatic Sciences (2004).             |
| Northern Gulf St<br>Lawrence        | 116                                       | Morissette, L., Despatie S.-P., Savenkoff, C., Hammill, M. O., Bourdages, H., Chabot, D. Data gathering and input parameters to construct ecosystem models for the northern Gulf of St. Lawrence (mid-1980s). Canadian Technical Report of Fisheries and Aquatic Sciences (2003). |

**References to the sources of empirical food webs used - continued from previous page**

| Name                    | Ecobase ID / Re-marks | Reference                                                                                                                                                                                                                                                                                                                                                                 |
|-------------------------|-----------------------|---------------------------------------------------------------------------------------------------------------------------------------------------------------------------------------------------------------------------------------------------------------------------------------------------------------------------------------------------------------------------|
| Northwest Africa        | 118                   | Morissette, L., Melgo, J. L., Kaschner, K., Gerber, L., Bamy, I. L. Food web model and data for studying the interactions between marine mammals and fisheries in the Northwest African ecosystem. Modelling the trophic role of marine mammals in tropical areas: data requirements, uncertainty, and validation. Fisheries Centre Research Reports 17 (2), 6-52 (2009). |
| Oneida Lake             | Pre                   | Miehls, A.L.J., Mason, D. M., Frank, K. A., Krause, A. E., Peacor, S. D., Taylor, W. W. Invasive species impacts on ecosystem structure and function: A comparison of the Bay of Quinte, Canada, and Oneida Lake, USA, before and after zebra mussel invasion. Ecological Modelling 220 (22), 3182–3193 (2009).                                                           |
|                         | Post                  |                                                                                                                                                                                                                                                                                                                                                                           |
| Bay of Quinte           | Pre                   |                                                                                                                                                                                                                                                                                                                                                                           |
|                         | Post                  |                                                                                                                                                                                                                                                                                                                                                                           |
| Orbetello Lagoon        | 232                   | Brando, V. E., Ceccarelli, R., Libralato, S., Ravagnan, G. Assessment of environmental management effects in a shallow water basin using mass-balance models. Ecological Modelling 172 (2-4), 213-232 (2004).                                                                                                                                                             |
| Oyster Reef             |                       | Dame, R. F., Patten, B. C. Analysis of energy flows in an intertidal oyster reef. Marine Ecology Progress Series 5 (2), 115-124 (1981).                                                                                                                                                                                                                                   |
| Paraná River Floodplain | 298                   | Angelini, R., Agostinho, A. A. Food web model of the Upper Paraná River Floodplain: description and aggregation effects. Ecological Modelling 181 (2-3), 109-121 (2005).                                                                                                                                                                                                  |
| Peru                    | 311                   | Jarre-Teichmann, A., Pauly, D. Seasonal Changes in the Peruvian Upwelling Ecosystem. Trophic models of aquatic ecosystems, 307-314 (1993).                                                                                                                                                                                                                                |
|                         | 312                   |                                                                                                                                                                                                                                                                                                                                                                           |
|                         | 658                   |                                                                                                                                                                                                                                                                                                                                                                           |
| Peru                    | 439                   | Guénette, S., Christensen, V., Pauly, D. Trophic modelling of the Peruvian upwelling ecosystem: Towards reconciliation of multiple datasets. Progress in Oceanography 79 (2-4), 326-335 (2008).                                                                                                                                                                           |
| Port Cros               | 497                   | Valls, A., Gascuel, D., Guénette, S., Francour, P. Modeling trophic interactions to assess the effects of a marine protected area: case study in the NW Mediterranean Sea. Marine Ecology Progress Series 456 201-201 (2012).                                                                                                                                             |
| Port Phillip Bay        | 431                   | Fulton, E. A., Smith, T. Ecosim Case Study: Port Phillip Bay, Australia. Fisheries Centre Research Reports 10 (2), 83-93 (2002).                                                                                                                                                                                                                                          |
| Prince William Sound    | 279                   | Okey, T. A., Wright, B. A. Toward ecosystem-based extraction policies for Prince William Sound, Alaska: integrating conflicting objectives and rebuilding Pinnipeds. Bulletin of Marine Science 74 (3), 727-747 (2004).                                                                                                                                                   |
| Raja Ampat              | 400                   | Pitcher, T. J., Ainsworth, C. H., Bailey, M. Ecological and economic analyses of marine ecosystems in the birds head seascape, Papua, Indonesia: I. Fisheries Centre Research 15 (5) (2007).                                                                                                                                                                              |
|                         | 401                   |                                                                                                                                                                                                                                                                                                                                                                           |

**References to the sources of empirical food webs used - continued from previous page**

| Name               | Ecobase ID / Re-marks | Reference                                                                                                                                                                                                                                                                       |
|--------------------|-----------------------|---------------------------------------------------------------------------------------------------------------------------------------------------------------------------------------------------------------------------------------------------------------------------------|
| Ria Formosa        | 125                   | Gamito, S., Erzini, K. Trophic food web and ecosystem attributes of a water reservoir of the Ria Formosa (south Portugal). Ecological Modelling 181 (4) 509-520 (2005).                                                                                                         |
| Santa Pola Bay     | 537                   | Bayle-Sempere, J. T., Arreguín-Sánchez, F., Sanchez-Jerez, P., Salcido-Guevara, L. A., Fernandez-Jover, D., Zetina-Rejón, M.J. Trophic structure and energy fluxes around a Mediterranean fish farm. Ecological Modelling 248, 135-147 (2013).                                  |
| Sechura Bay        | 489                   | Taylor, M. H., Wolff, M., Vadas, F., Yamashiro, C. Trophic and environmental drivers of the Sechura Bay Ecosystem over an ENSO cycle. . Helgoland Marine Research 62 (1), 15-32 (2008). (Peru).                                                                                 |
| Senegambia         | 133                   | Samb, B., Mendy, A. Dynamique du réseau trophique de lécosystème sénégalais en 1990 West African marine ecosystems: models and fisheries impacts. Fisheries Centre Research Reports 12, 57-70 (2004).                                                                           |
| Sierra Leone       | 135                   | Heymans, J. J., Vakily, J. M. Structure and dynamics of the marine ecosystem off Sierra Leone for three time periods: 1964, 1978, 1990. West African marine ecosystems: models and fisheries impacts. Fisheries Centre Research Reports 12, 160-169 (2004).                     |
|                    | 137                   |                                                                                                                                                                                                                                                                                 |
|                    | 136                   |                                                                                                                                                                                                                                                                                 |
| Sinaloa sur Mexico | 325                   | Salcido Guevara, L. A., Estructura y flujos de biomasa en un ecosistema bentónico explotado en el Sur de Sinaloa, Mexico. Doctoral dissertation, Instituto Politécnico Nacional. Centro Interdisciplinario de Ciencias Marinas (2006).                                          |
| Somme Estuary      |                       | Rybarczyk, H., Laboratoire Hydrobiologie, UPMC, 12 Rue Cuvier 75252. Paris Cedex 05                                                                                                                                                                                             |
| Sonda de Campeche  | 240                   | Manickchand-Heileman, S., Soto, L. A. Escobar, E. A Preliminary Trophic Model of the Continental Shelf, South-western Gulf of Mexico. Estuarine, coastal and shelf Science 46 (6), 885-899 (1998).                                                                              |
| Sonda Campeche Act | 291                   | Zetina-Rejón, M. J., Arreguín-Sánchez, F., Flujos de energía y estructura trófica de la Sonda de Campeche, Suroeste del Golfo de México. Memorias del III Foro de Camarón del Golfo de México y del Mar Caribe. INP-SAGARPA y Gob. del Estado de Campeche, México 49-57 (2003). |
| Sørfjord           | 429                   | Falk-Petersen, J. Ecosystem effects of red king crab invasion - a modelling approach using Ecopath with Ecosim. Master's thesis, Universitetet i Tromsø (2004).                                                                                                                 |
| South Benguela     | 485                   | Shannon, L. J., Moloney, C. L., Jarre, A., Field, J. G. Trophic flows in the southern Benguela during the 1980s and 1990s. Journal of Marine Systems 39 (1-2), 83-116 (2003).                                                                                                   |
| South Benguela     | 504                   | Watermeyer, K. E., Shannon, L. J., Griffiths, C. L. Changes in the trophic structure of the southern Benguela before and after the onset of industrial fishing. African Journal of Marine Science 30 (2), 351-382 (2008).                                                       |
|                    | 505                   |                                                                                                                                                                                                                                                                                 |
| South of Benguela  | 506                   |                                                                                                                                                                                                                                                                                 |

**References to the sources of empirical food webs used - continued from previous page**

| <b>Name</b>                             | <b>Ecobase<br/>ID /<br/>Re-<br/>marks</b> | <b>Reference</b>                                                                                                                                                                                                                                                                                                 |
|-----------------------------------------|-------------------------------------------|------------------------------------------------------------------------------------------------------------------------------------------------------------------------------------------------------------------------------------------------------------------------------------------------------------------|
| South Shetlands                         | 663                                       | Bredesen, E. L. Krill and the Antarctic: Finding the Balance. Doctoral dissertation, University of British Columbia (2003).                                                                                                                                                                                      |
| South West Viet-<br>nam                 | 415                                       | Christensen, V., Garces, L. R., Silvestre, G. T., Pauly, D. Fisheries impact on the South China Sea Large Marine Ecosystem: a preliminary analysis using spatially explicit methodology. World Fish Center Conference Proceedings 67, 51-62 (2003).                                                              |
| West Coast<br>of Peninsular<br>Malaysia | 414                                       |                                                                                                                                                                                                                                                                                                                  |
| South western<br>Gulf of Mexico         | 687                                       | Arreguin-Sánchez, F., Valero-Pacheco, E., Chavez, E. A. A trophic box model of the coastal fish communities of the southwestern Gulf of Mexico. Trophic models of aquatic ecosystems. ICLARM Conf. Proc 26, 197-205 (1993).                                                                                      |
| Southern Brazil                         | 664                                       | Vasconcellos, M., Gasalla, M. A. Fisheries catches and the carrying capacity of marine ecosystems in southern Brazil. Fisheries Research 50 (3), 279-295 (2001).                                                                                                                                                 |
| Southern Gulf of<br>St. Lawrence        | 145                                       | Savenkoff, C., Bourdages, H., Swain, D. P., Despatie, S.-P., Hanson, M. J., Méthot, R., Morissette, L., Hammill M.O. Input data and parameter estimates for ecosystem models of the southern Gulf of St. Lawrence (mid-1980s and mid-1990s). Canadian Technical Report of Fisheries and Aquatic Sciences (2004). |
| Sri Lanka                               | 441                                       | Haputhantri, S.S.K., Villanueva, M.C.S., Moreau, J. Trophic interactions in the coastal ecosystem of Sri Lanka: An ECOPATH preliminary approach. Estuarine, coastal and shelf science 76 (2), 304-318 (2008).                                                                                                    |
| St Marks                                | febs1                                     | Baird, D., Luczkovich, J., Christian, R. R. Assessment of spatial and temporal variability in ecosystem attributes of the St Marks national wildlife refuge, Apalachee Bay, Florida. Estuarine, Coastal and Shelf Science 47 (3) (1998). doi:10.1006/ecss.1998.0360                                              |
|                                         | febs2                                     |                                                                                                                                                                                                                                                                                                                  |
|                                         | febs4                                     |                                                                                                                                                                                                                                                                                                                  |
|                                         | January<br>Site 1                         |                                                                                                                                                                                                                                                                                                                  |
|                                         | January<br>Site 2                         |                                                                                                                                                                                                                                                                                                                  |
|                                         | January<br>Site 3                         |                                                                                                                                                                                                                                                                                                                  |

**References to the sources of empirical food webs used - continued from previous page**

| <b>Name</b>                           | <b>Ecobase ID / Re-marks</b> | <b>Reference</b>                                                                                                                                                                                                                                                                                                                             |
|---------------------------------------|------------------------------|----------------------------------------------------------------------------------------------------------------------------------------------------------------------------------------------------------------------------------------------------------------------------------------------------------------------------------------------|
| Strait of Gergia                      | 328                          | Martell, S. J. D., Beattie, A. I., Walters, C. J., Nayar, T., Briese, R. Simulating fisheries management strategies in the Strait of Georgia ecosystem using Ecopath and Ecosim The Use of Ecosystem Models to Investigate Multispecies Management Strategies for Capture Fisheries. Fisheries Centre Research Reports 10 (2), 16-23 (2002). |
| Tamiahua                              | 318                          | Abarca-Arenas, L. G., Valero-Pacheco, E. Toward a Trophic Model of Tamiahua, a Coastal Lagoon in Mexico. Trophic models of aquatic ecosystems. ICLARM Conf. Proc. 26, 181-185 (1993).                                                                                                                                                        |
| Tasmanian Seamounts Marine Reserve    | 407                          | Bulman, C. M., Butler, A. J., Condie, S. A trophodynamic model for the Tasmanian Seamounts Marine Reserve: links between pelagic and deepwater ecosystems. Report to CSIRO Marine Research Environment Australia and the Fisheries Research and Development Corporation (2002).                                                              |
| Tasmanian waters                      | 703                          | Watson, R. A., Nowara, G. B., Tracey, S. R., Fulton, E. A., Bulman, C. M., Edgar, G.J., Barrett, N.S., Lyle, J.M., Frusher, S.D., Buxton, C.D. Ecosystem model of Tasmanian waters explores impacts of climate-change induced changes in primary productivity. Ecological modelling 264, 115-129 (2013).                                     |
| Terminos Lagoon                       | 243                          | Manickchand-Heileman, S., Arreguin-Sánchez, F., Lara-Domínguez, A., Soto, L. A. Energy flow and network analysis of Terminos Lagoon, SW Gulf of Mexico . Journal of Fish Biology 53, 179-197 (1998).                                                                                                                                         |
| Thau                                  | 217                          | Palomares, M. L. D., Reyes-Marchant, P., Lair, N., Zainure, M., Barnabé, G., Lasserre, G. A Trophic Model of a Mediterranean Lagoon, Etang de Thau, France . 224-229 (1993).                                                                                                                                                                 |
| Upper Chesapeake Bay                  | Summer                       | Hagy, J. D. Eutrophication, hypoxia and trophic transfer efficiency in Chesapeake Bay. PhD Dissertation, University of Maryland at College Park (USA), 446 (2002).                                                                                                                                                                           |
| USA, Mid Atlantic Bight               | 99                           | Okey, T. A. A straw-man Ecopath model of the Middle Atlantic Bight continental shelf, United States. Fisheries Impacts on North Atlantic Ecosystems: Models and Analyses. Fisheries Centre Research Reports, 9 (4), 151-166 (2001).                                                                                                          |
| USA, South Atlantic Continental Shelf | 467                          | Okey, T. A., Pugliese, R. A preliminary Ecopath model of the Atlantic continental shelf adjacent to the Southeastern United States. Fisheries Impacts on North Atlantic Ecosystems: Models and Analyses. Fisheries Centre Research Reports, 9 (4), 167-181 (2001).                                                                           |
| Venezuela shelf                       | 282                          | Mendoza, J. J. A preliminary biomass budget for the Northeastern Venezuela shelf ecosystem. Trophic models of aquatic ecosystems 26, 285-297 (1993).                                                                                                                                                                                         |
| Virgin Islands                        | 324                          | Opitz, S. Trophic Interactions in Caribbean Coral Reefs. ICLARM Tech. Rep. 43, 341 p. (1996).                                                                                                                                                                                                                                                |
| West Coast of Sabah                   | 305                          | Garces, L. R., Man, A., Ahmad, A. T., Mohamad-Norizam, M., Silvestre, G. T. A trophic model of the coastal fisheries ecosystem off the West Coast of Sabah and Sarawak, Malaysia. WorldFish Center Conference Proceedings 67, 333-352 (2003).                                                                                                |
